# Supplementary material for: Chladni states in Ising Spin Lattices
Source: arXiv:2507.05961 source file (2026-10-05)
Supplement: Supplementary file 1 [file Supplemental_Material_Chladni.pdf]

# Chladni states in Ising Spin Lattices

Giulio Iannelli[1, 2, *] and Pablo Villegas[1, 3, †]

[1] *'Enrico Fermi' Research Center (CREF), Via Panisperna 89A, 00184 - Rome, Italy*
[2] *Dipartimento di Fisica, Università degli Studi di Palermo, 90133 Palermo, Italy*
[3] *Instituto Carlos I de Física Teórica y Computacional, Univ. de Granada, E-18071, Granada, Spain.*

## CONTENTS

Hubbard-Stratonovich transformation and discrete Laplacian eigenstates 2

Chladni states in 2D lattices 3
Square lattice 3
Triangular lattice 6
Hexagonal lattice 9
Supercrystal lattice 12

Frustrated antiferromagnetic lattices at zero temperature. 14

Spin-glass systems 16

Topological reconstruction of images 17

References 20

* giulio.iannelli@cref.it
† pablo.villegas@cref.it

## HUBBARD-STRATONOVICH TRANSFORMATION AND DISCRETE LAPLACIAN EIGENSTATES

Without loss of generality, we recover the calculation performed in [1] to tighten the relation between the fundamental state of the signed Laplacian[1], $\bar{L} = |D| - A$ and the ground state of the Ising Hamiltonian in the general case of an arbitrary interaction matrix $J_{ij}$. It is convenient to introduce the field theoretical formulation of the Ising model given by the Hubbard-Stratonovich transformation (we refer to [2, 3] for a detailed description on the issue), namely,

$$Z(J) = \sum_{\boldsymbol{\sigma}} e^{-\beta \mathscr{H}[\boldsymbol{\sigma}]} \propto \int \mathcal{D}\phi \, \exp\left\{ -\beta \sum_{(i,j)} J_{ij}\phi_i\phi_j + \sum_i \ln\left[\cosh\left(2\beta \sum_j J_{ij}\phi_j\right)\right]\right\}, \tag{1}$$

where $\beta = 1/T$ and $\mathcal{D}\phi = \prod_i d\phi_i$. For $\beta \to +\infty$ we can apply the saddle-point method, leading to the self-consistent equations for the ground state:

$$\sum_i J_{ki}\left(\phi_i - \text{sign}\left[\sum_l A_{il}\phi_l\right]\right) = 0,$$

for $k = 1, 2, ...., N$, where $A_{ij} = J_{ij}/J$ is the adjacency matrix of the network of interactions. The self-consistent solution of the above equation is

$$\phi_i = \text{sign}\left[\sum_l A_{il}\phi_l\right]. \tag{2}$$

Note that, as expected, for the case $p = 0$, this gives two specular ferromagnetic solutions, either $\phi_i = +1$ or $\phi = -1$ for all $i$. Now $p$ corresponds to the fraction of negative links as defined in the random bond Ising model (see [1] for further details). The symmetry can be broken either by a small and uniform external magnetic field or by suitable boundary conditions. At small $p \neq 0$, two ferromagnetic ground states related by the same global up-down symmetry are still present, but they are no longer homogeneous due to the inhomogeneous pair interactions. When instead $p$ becomes large enough, i.e. at the $T = 0$ critical value $p_c$, the ferromagnetic ground state is no longer unique. Still, many different and degenerate ground states are solutions of Eq. (2), and a spin glass transition appears.

Let us now see the relation between the solutions of Eq. (2) and the eigenvector(s) related to the least eigenvalue of $\bar{L}$. As aforementioned, it (they) satisfies the following equation

$$\sum_{i=1}^{N} \bar{L}_{ij}\psi_j = \lambda_0\psi_i\,,$$

which can also be rewritten as

$$\sum_{i=1}^{N} A_{ij}\psi_j = (k_i - \lambda_0)\psi_i\,, \tag{3}$$

where $k_i = \sum_j |A_{ij}|$ is the coordination number of site $i$ ($k_i = 2d$ for a $d-$dimensional square lattice). As shown in [4], $\lambda_0 \leq \min_{i=1}^{N} k_i$. This implies that for all connected networks, including regular lattices:

$$\text{sign}[\psi_i] = \text{sign}\left[\sum_l A_{il}\psi_l\right]. \tag{4}$$

Eq. (4) is formally the same of Eq. (2) with the fundamental difference that the solution of the former has to be found on the $N-$dimensional spherical surface of radius $\sqrt{N}$ while for the latter has to found on the vertices of the $N-$dimensional cube defined by $\phi_i = \pm 1$ for each $i = 1, 2, ..., N$ (note however that in both cases $|\boldsymbol{\psi}| = |\boldsymbol{\phi}| = \sqrt{N}$. This implies that sign$[\psi_i]$ can differ from sign$[\phi_i]$ in some node in particular where there are large fluctuations in the values of $\psi$ between neighboring nodes. Anyway, being $\boldsymbol{\phi}$ and $\boldsymbol{\psi}$ characterized by the same normalization condition, we expect that the binarized vector $\boldsymbol{\psi}_{\text{bin}}$ of components $\psi_i/|\psi_i|$ shows a similar behavior with respect the binary vector $\boldsymbol{\phi}$ on a suitable coarse-grained scale as large as the frustration walls.

---

[1] This choice allows us to tackle the most general case for any Ising spin lattice, as $\bar{L}$ is formally equal to the Laplacian matrix, $L = D - A$, when all the entries have positive weights.

**CHLADNI STATES IN 2D LATTICES**

**Square lattice**

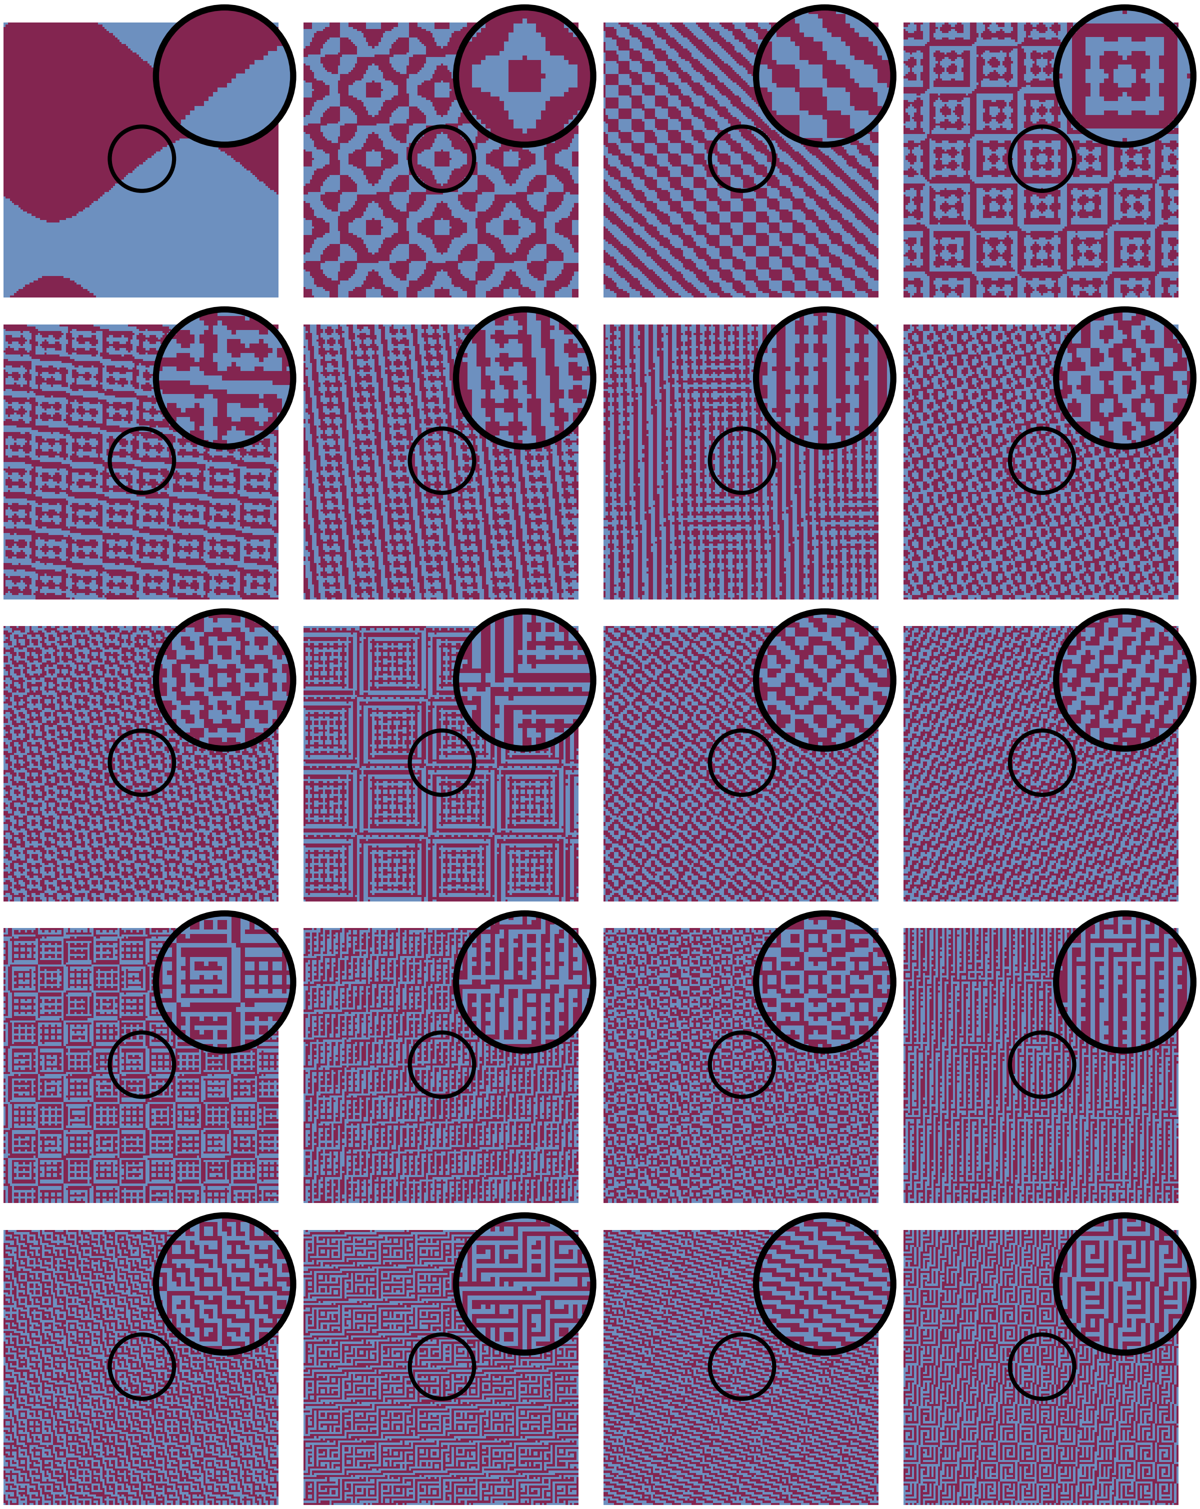

Figure 1. Chladni states for a 2D square lattice with side $L = 128$ associated with different eigenvectors (in order, from top left corner to bottom right one: {1, 432, 863, 1294, 1725, 2156, 2587, 3018, 3449, 3880, 4312, 4743, 5174, 5605, 6036, 6467, 6898, 7329, 7760, 8192}. Zoomed regions illustrate the microscopic structure of complex patterns and different domain walls.

Figure 2 reports the combination of different Chladni states $\widetilde{|\lambda_i\rangle} \equiv \mathrm{sign}(|\lambda_i\rangle)$ (we will omit the long tilde in figures caption for the sake of clarity) via weighted sum

$$|w\rangle = \sum_i c_i \widetilde{|\lambda_i\rangle}$$

and their temporal evolution using zero-temperature kinetically constrained dynamics. As a technical remark, we emphasize that the weighted sum can produce zero values at particular nodes– because of the discreteness of the state space, where the indeterminate value needs to be fixed, e.g., to one. Pay close attention to how the system retains some memory regarding the initial state when patterns evolve (see, for instance, the purple line in Fig. 2). Note also that the decay to an equilibrium state depend on the original combination of Chladni states (see red line in Fig. 2). Notably, the system retains memory of the initial state only in those parts of the system that belong to Chladni states with negative energy. In particular, we show how the direct combination of Chladni states with negative energy generates new stable solutions of the Ising spin lattice at zero temperature.

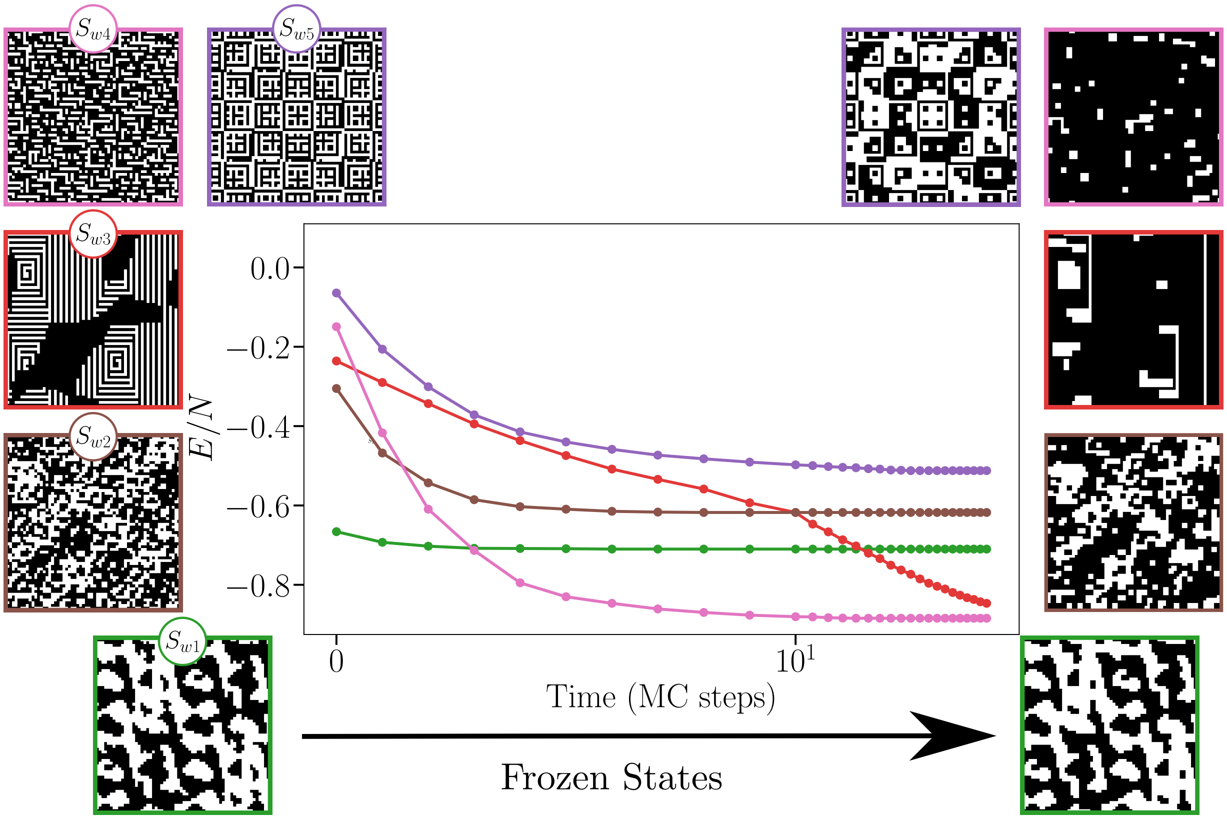


Figure 2. Temporal evolution and snapshots of the composition with weights of Chladni states for the square lattice of size $N = L^2 = 4096$. The different states consist of the following combinations: $|S_{w1}\rangle = {}^{1}/_{10}\,|\lambda_8\rangle + {}^{3}/_{10}\,|\lambda_{32}\rangle + {}^{2}/_{5}\,|\lambda_{128}\rangle + {}^{1}/_{5}\,|\lambda_{256}\rangle$, $|S_{w2}\rangle = {}^{3}/_{25}\,|\lambda_8\rangle + {}^{9}/_{40}\,|\lambda_{33}\rangle + \cdots + {}^{3}/_{25}\,|\lambda_{1046}\rangle + {}^{9}/_{50}\,|\lambda_{1086}\rangle$, $|S_{w3}\rangle = {}^{1}/_{5}\,|\lambda_8\rangle + {}^{3}/_{10}\,|\lambda_{16}\rangle + {}^{1}/_{2}\,|\lambda_{1982}\rangle$, $|S_{w4}\rangle = {}^{1}/_{5}\,|\lambda_{568}\rangle + {}^{3}/_{10}\,|\lambda_{876}\rangle + {}^{1}/_{2}\,|\lambda_{1952}\rangle$ and $|S_{w5}\rangle = {}^{2}/_{5}\,|\lambda_{18}\rangle + {}^{3}/_{5}\,|\lambda_{1684}\rangle$.

Figure 3 reports the combination of different Chladni states by using the element-wise product

$$|p\rangle = \bigodot_i |\lambda_i\rangle$$

where $(|a\rangle \odot |b\rangle)_i = a_i \cdot b_i$. This is equivalent to the dot product for the $(\mathbb{Z}_2)^N \cong (\{\pm 1\}^N, \odot)$ group.

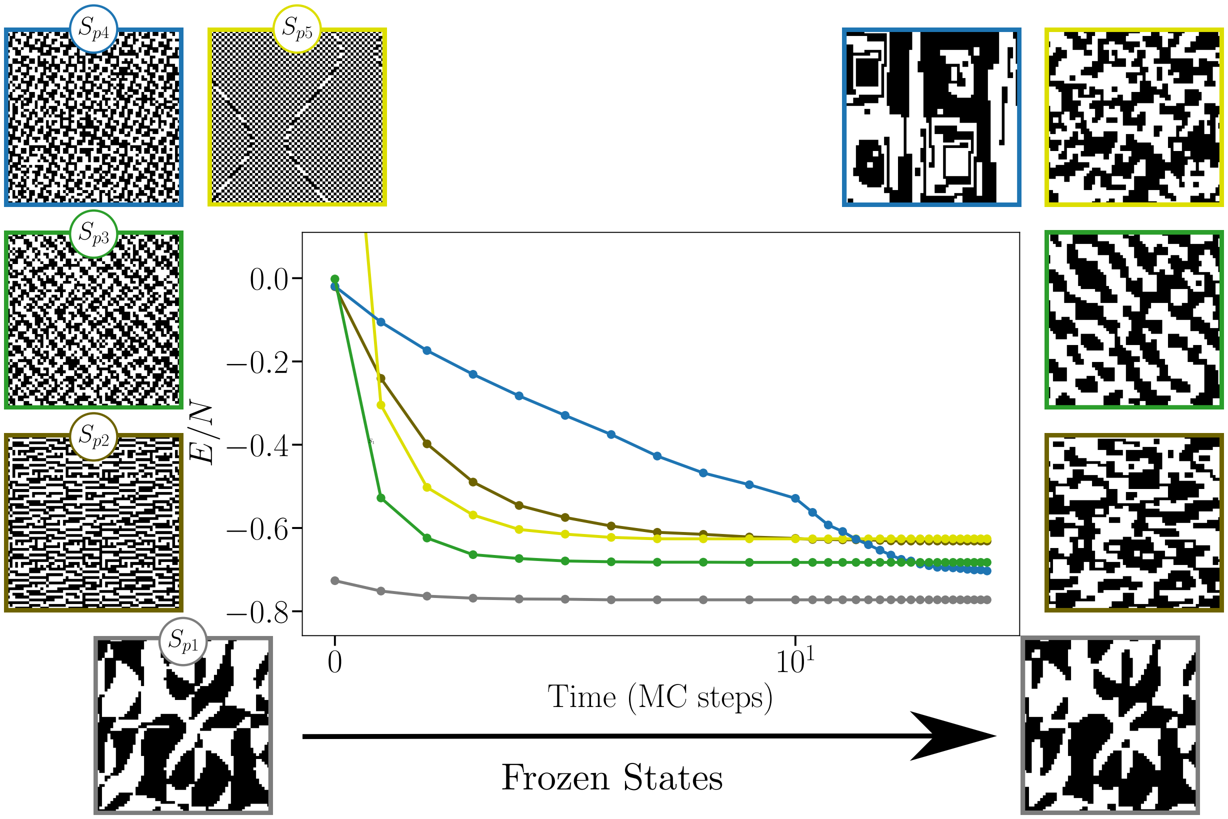


Figure 3. Temporal evolution and snapshots of the composition by element-wise product of Chladni states for the square lattice of size $N = L^2 = 4096$. The different states consist of the following combinations: $|S_{p1}\rangle = |\lambda_8\rangle \odot |\lambda_{16}\rangle \odot |\lambda_{32}\rangle$, $|S_{p2}\rangle = |\lambda_{64}\rangle \odot |\lambda_{2155}\rangle$, $|S_{p3}\rangle = |\lambda_{1836}\rangle \odot |\lambda_{1984}\rangle$, $|S_{p4}\rangle = |\lambda_4\rangle \odot |\lambda_{16}\rangle \odot |\lambda_{1982}\rangle$ and $|S_{p5}\rangle = |\lambda_4\rangle \odot |\lambda_{4095}\rangle$.

**Triangular lattice**

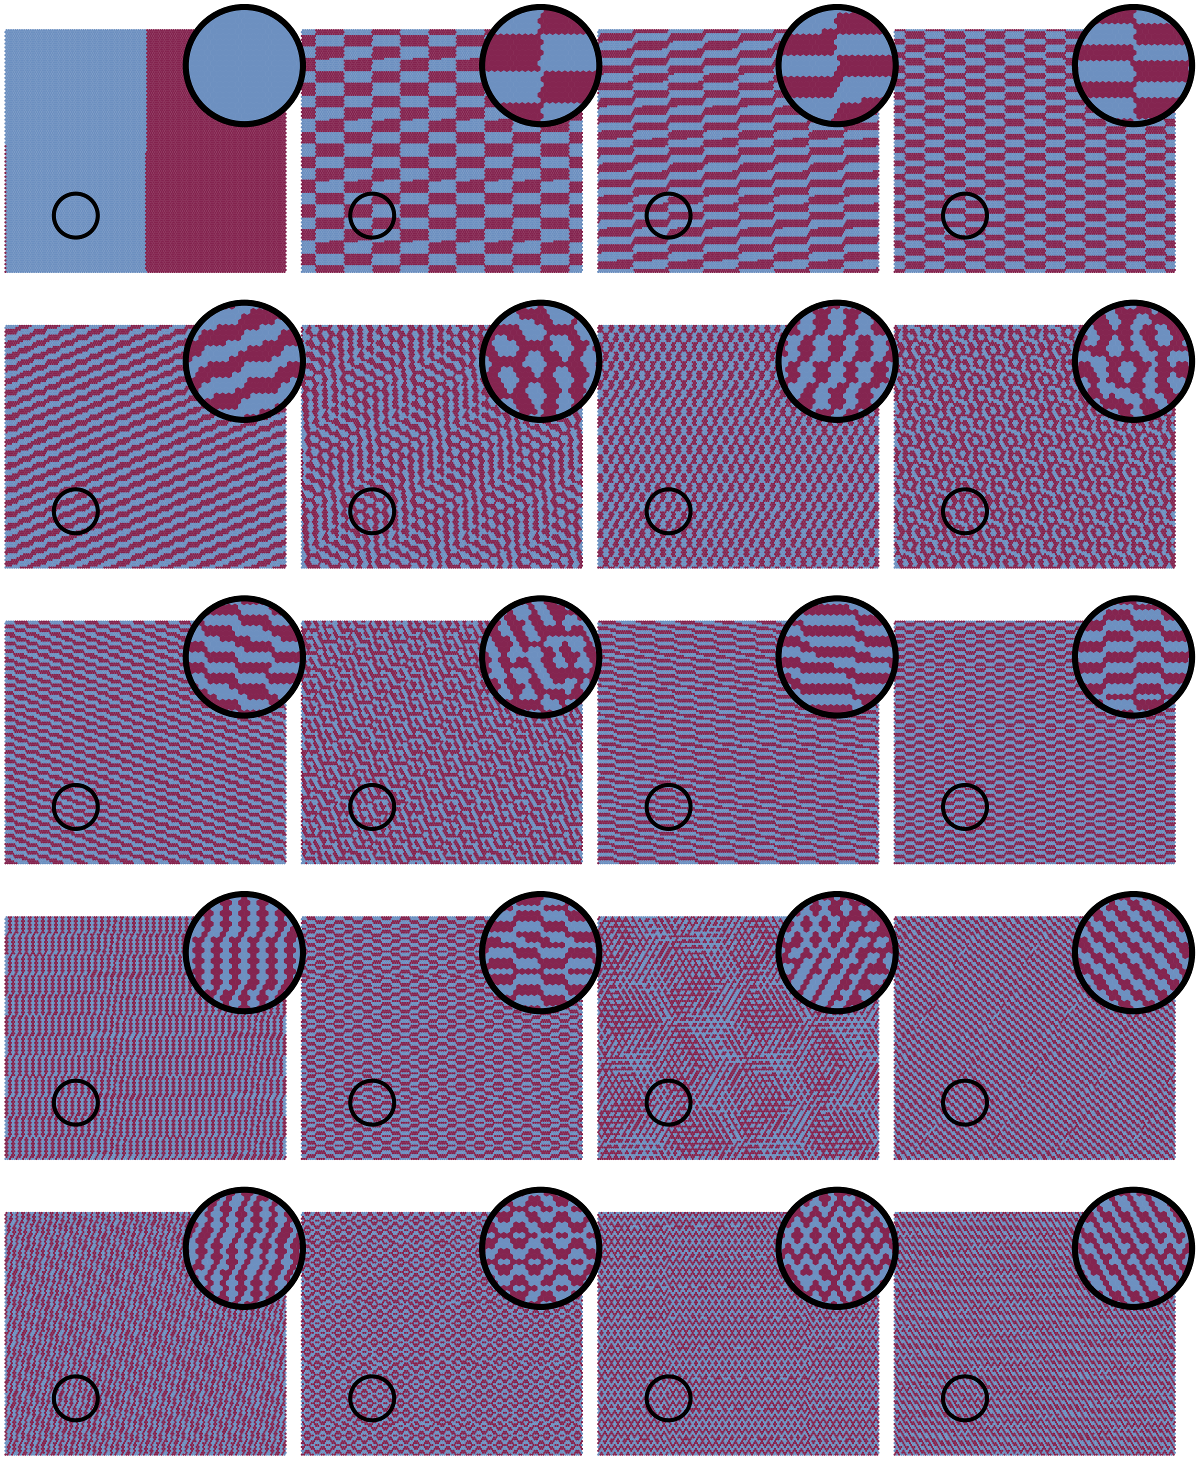

Figure 4. Chladni states for a 2D triangular lattice with side $L = 128$ associated with different eigenvectors (see title). (in order, from top left corner to bottom right one: {1, 432, 863, 1294, 1725, 2156, 2587, 3018, 3449, 3880, 4312, 4743, 5174, 5605, 6036, 6467, 6898, 7329, 7760, 8192}. Zoomed regions illustrate the microscopic structure of complex patterns and different domain walls.

Figure 5 shows the energy corresponding to each normalized Chladni state as a function of the normalized growing eigenvectors for a 2D triangular lattice, being independent of the system size. Note that the energy curve does not exhibit symmetry about the origin, as a consequence of the lack of an antiferromagnetic phase in this case. Again, Chladni states with negative energy are stable over time at $T = 0$.

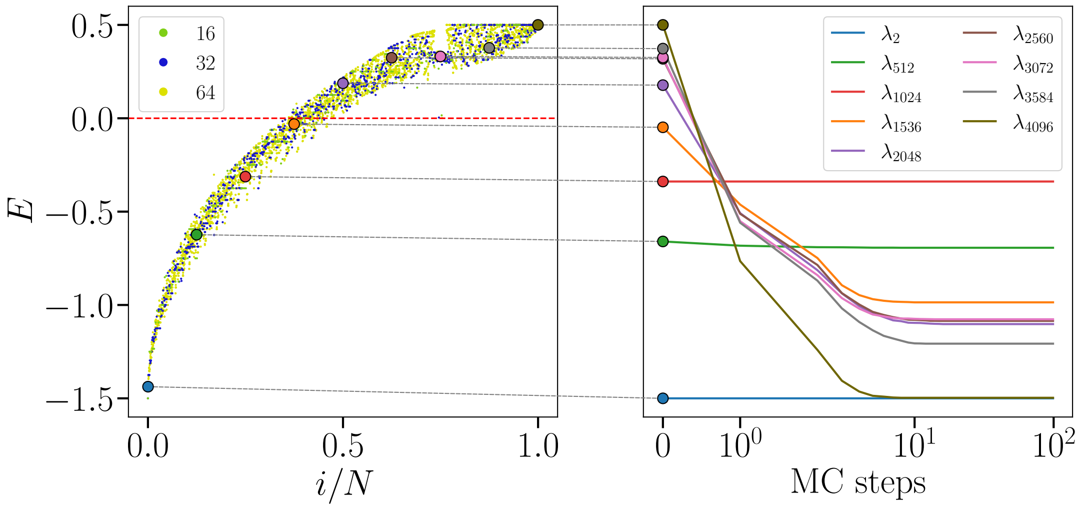


Figure 5. **Chladni states in 2D triangular lattices.** **(Left)** Ising energy versus normalized eigenstate number for different system sizes (see legend, $N = L^2$). Note the natural collapse of the curve for all lattice sizes. The red dashed line indicates zero energy. **(Right)** Temporal evolution at $T = 0$ of the different Chladni states versus time (in MC steps) for selected configurations (see legend) and energy mapping (dashed lines). Chladni states with enough negative energy define stable configurations over time.

Figure 6 reports the combination of different Chladni states $\widetilde{|\lambda_i\rangle}$ for the 2D triangular lattice via weighted sum, $|w\rangle = \sum_i c_i |\lambda_i\rangle$, and their temporal evolution considering the kinetically-constrained dynamics at zero temperature. During evolution, the system retains memory of structures stemming from negative-energy regions (see, for instance, the brown line in Fig. 6). Note that the decay to an equilibrium state depends on the original combination of Chladni states (see red line in Fig. 6).

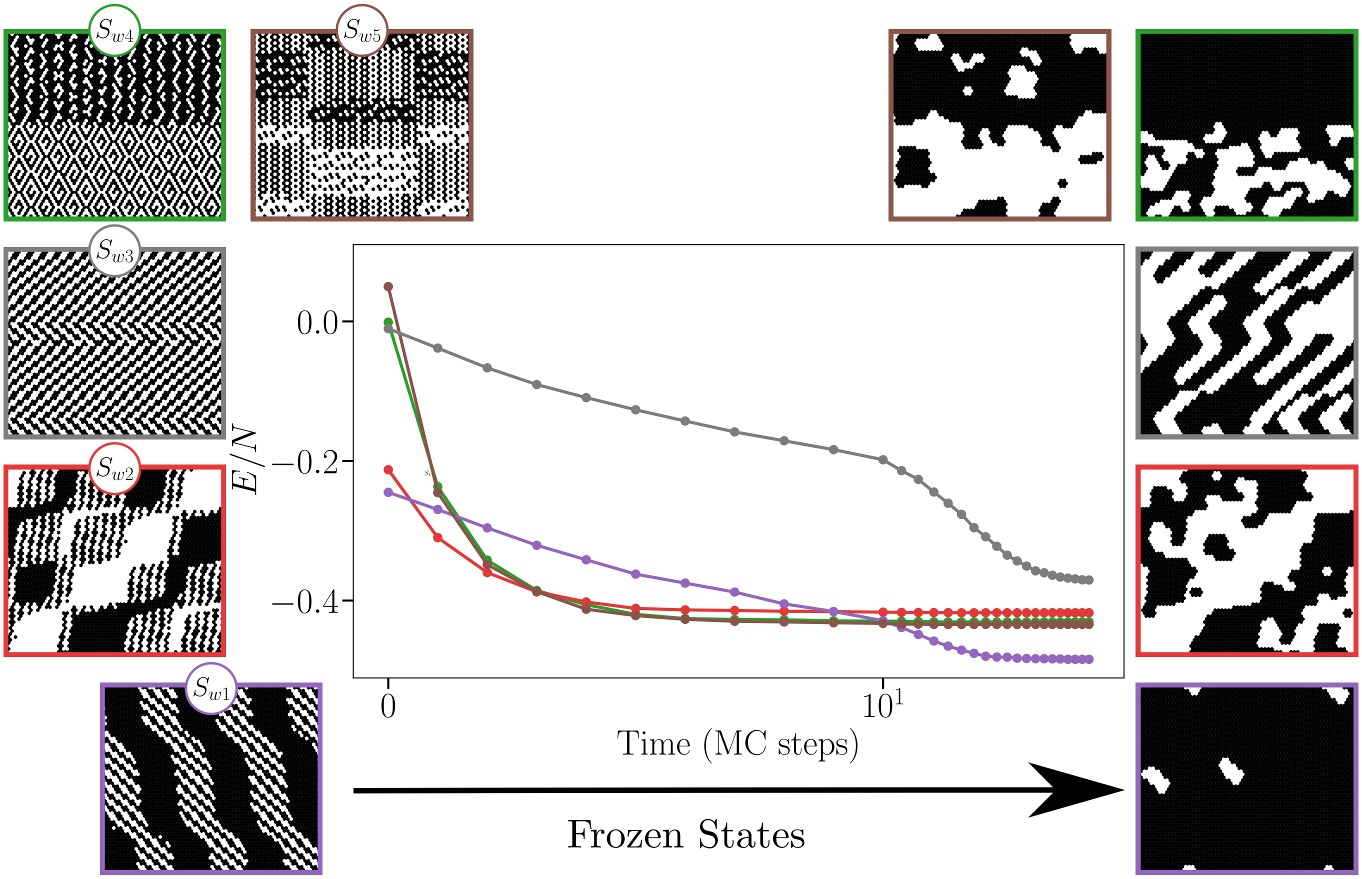


Figure 6. Temporal evolution and snapshots of the composition with weights of Chladni states for the triangular lattice of size $N = L^2 = 4096$. The different states consist of the following combinations: $|S_{w1}\rangle = {}^1\!/\!_2\,|\lambda_{27}\rangle + {}^1\!/\!_2\,|\lambda_{1521}\rangle$, $|S_{w2}\rangle = {}^3\!/\!_{10}\,|\lambda_6\rangle + {}^1\!/\!_4\,|\lambda_{24}\rangle + {}^9\!/\!_{20}\,|\lambda_{1756}\rangle$, $|S_{w3}\rangle = 1\,|\lambda_{1522}\rangle$, $|S_{w4}\rangle = {}^1\!/\!_5\,|\lambda_4\rangle + {}^3\!/\!_{10}\,|\lambda_{612}\rangle + {}^1\!/\!_2\,|\lambda_{3192}\rangle$ and $|S_{w5}\rangle = {}^3\!/\!_5\,|\lambda_4\rangle + {}^1\!/\!_5\,|\lambda_{18}\rangle + {}^1\!/\!_5\,|\lambda_{2560}\rangle + {}^2\!/\!_5\,|\lambda_{3894}\rangle$.

**Hexagonal lattice**

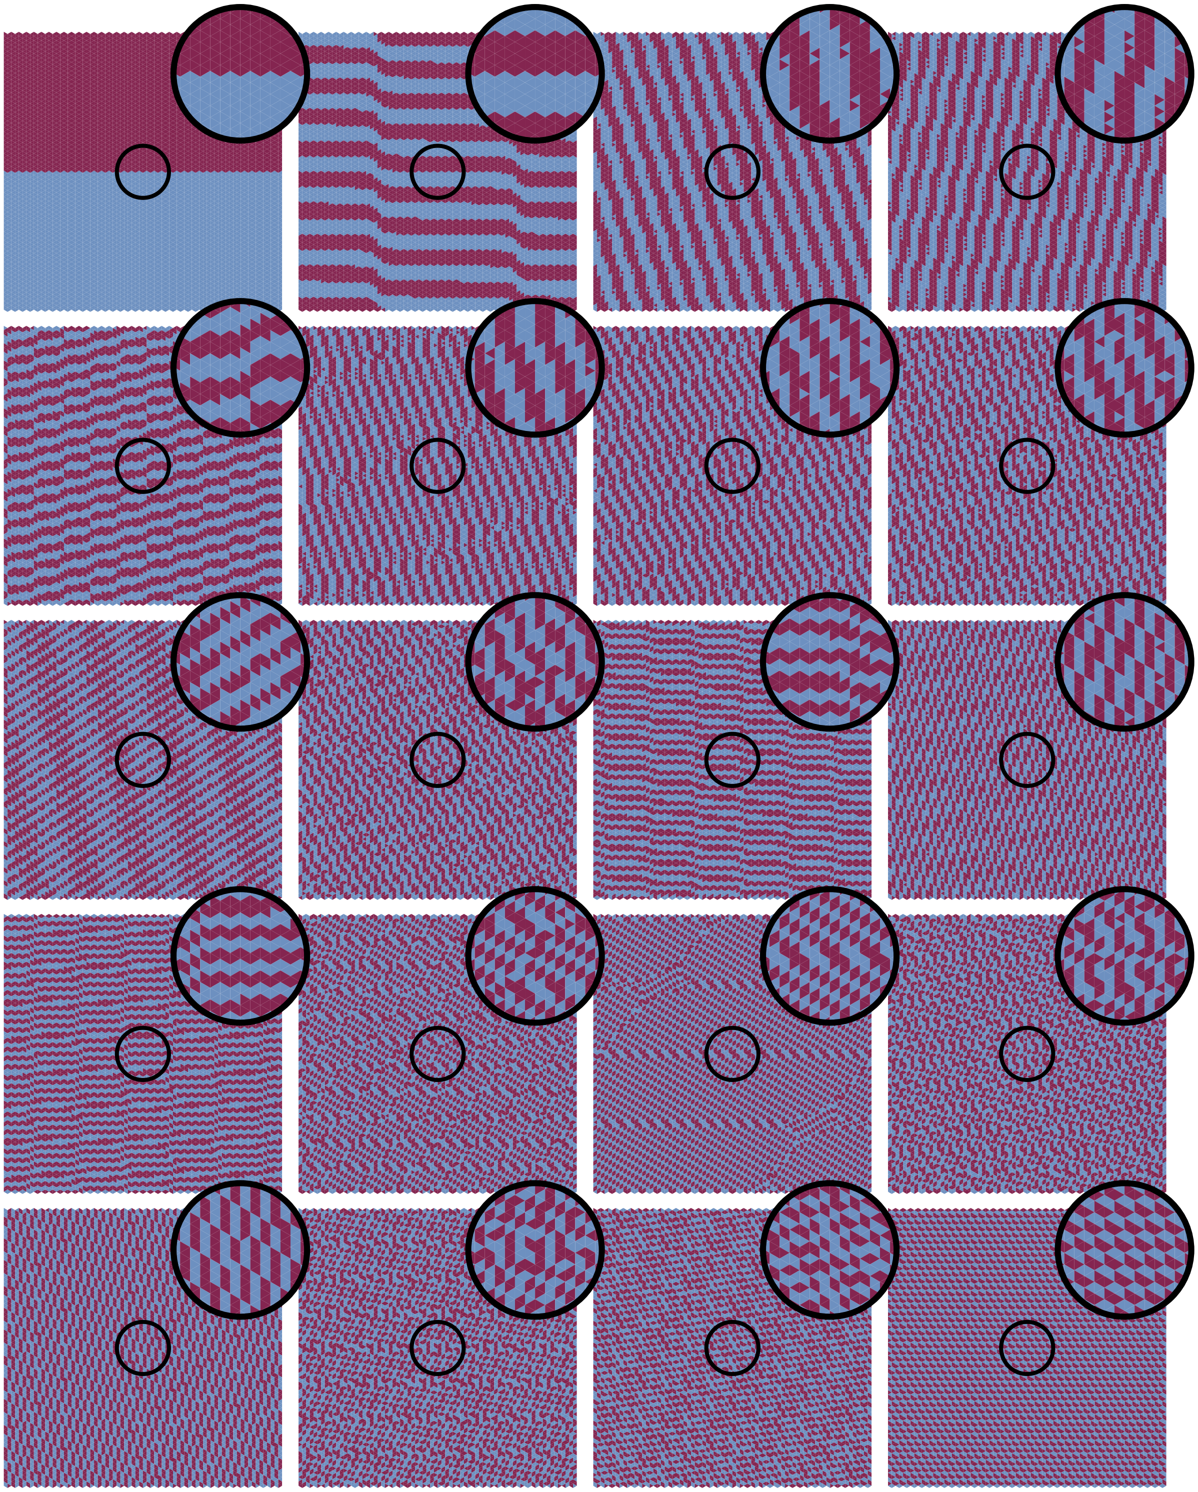

Figure 7. Chladni states for a 2D hexagonal lattice of size $N = L_1 \cdot L_2$, with sides $L_1 = 128, L_2 = 74$, associated with different eigenvectors (in order, from top left corner to bottom right one: $\{1$, 250, 499, 748, 997, 1247, 1496, 1745, 1994, 2243, 2493, 2742, 2991, 3240, 3489, 3739, 3988, 4237, 4486, $4736\}$. Zoomed regions illustrate the microscopic structure of complex patterns and different domain walls.

Figure 8 shows the energy corresponding to each normalized Chladni state as a function of the normalized growing eigenvectors. The energy curve exhibits a characteristic double S-shape, independent of system size, and is symmetric about the origin, as expected due to the existence of an antiferromagnetic phase. We have performed extensive Monte Carlo simulations of selected Chaldni states at $T = 0$ to monitor their temporal evolution and analyze their stability, as reported in Fig. 8. In particular, we observe that such states associated with low lattice eigenmodes (or large spatial scales) exhibit negative energy and are temporally stable, i.e., the system remains stuck.

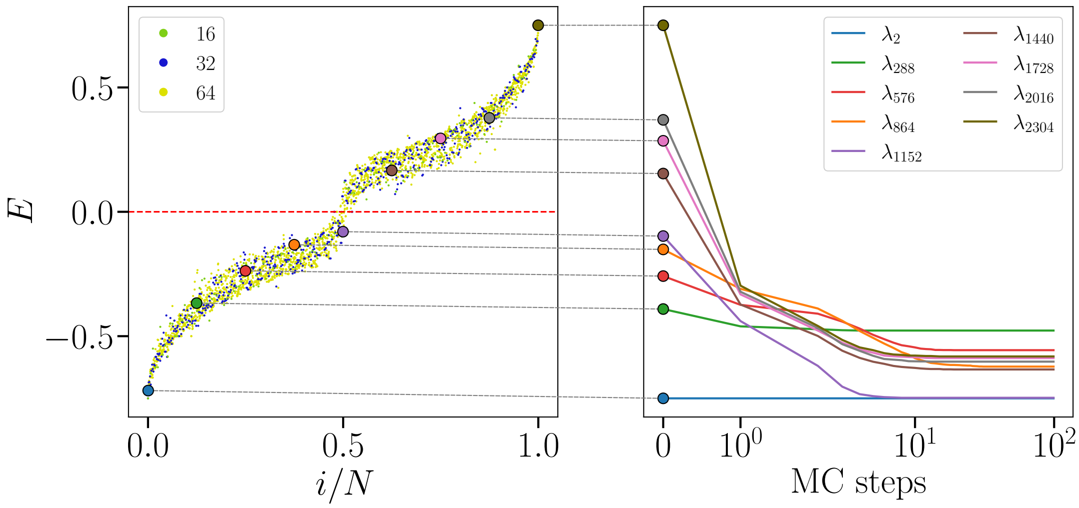


Figure 8. **Chladni states in 2D hexagonal lattices. (Left)** Ising energy versus normalized eigenstate number for different system sizes (see legend, $N = L^2$). Note the natural curve collapse for all lattice sizes with an inversion point at half the system size, separating the positive from the negative energy region. The red dashed line indicates zero energy. **(Right)** Temporal evolution at $T = 0$ of the different Chladni states versus time (in MC steps) for selected configurations (see legend) and energy mapping (dashed lines). Chladni states with enough negative energy define stable configurations over time.

Figure 9 reports the combination of different Chladni states $\widetilde{|\lambda_i\rangle}$ for the 2D hexagonal lattice via weighted sum, $|w\rangle = \sum_i c_i |\lambda_i\rangle$, and their temporal evolution considering the kinetically-constrained dynamics at zero temperature. During evolution, the system retains memory of structures stemming from negative-energy regions (see, for instance, the pink line in Fig. 9). Note that the decay to an equilibrium state depends on the original combination of Chladni states (see orange line in Fig. 9).

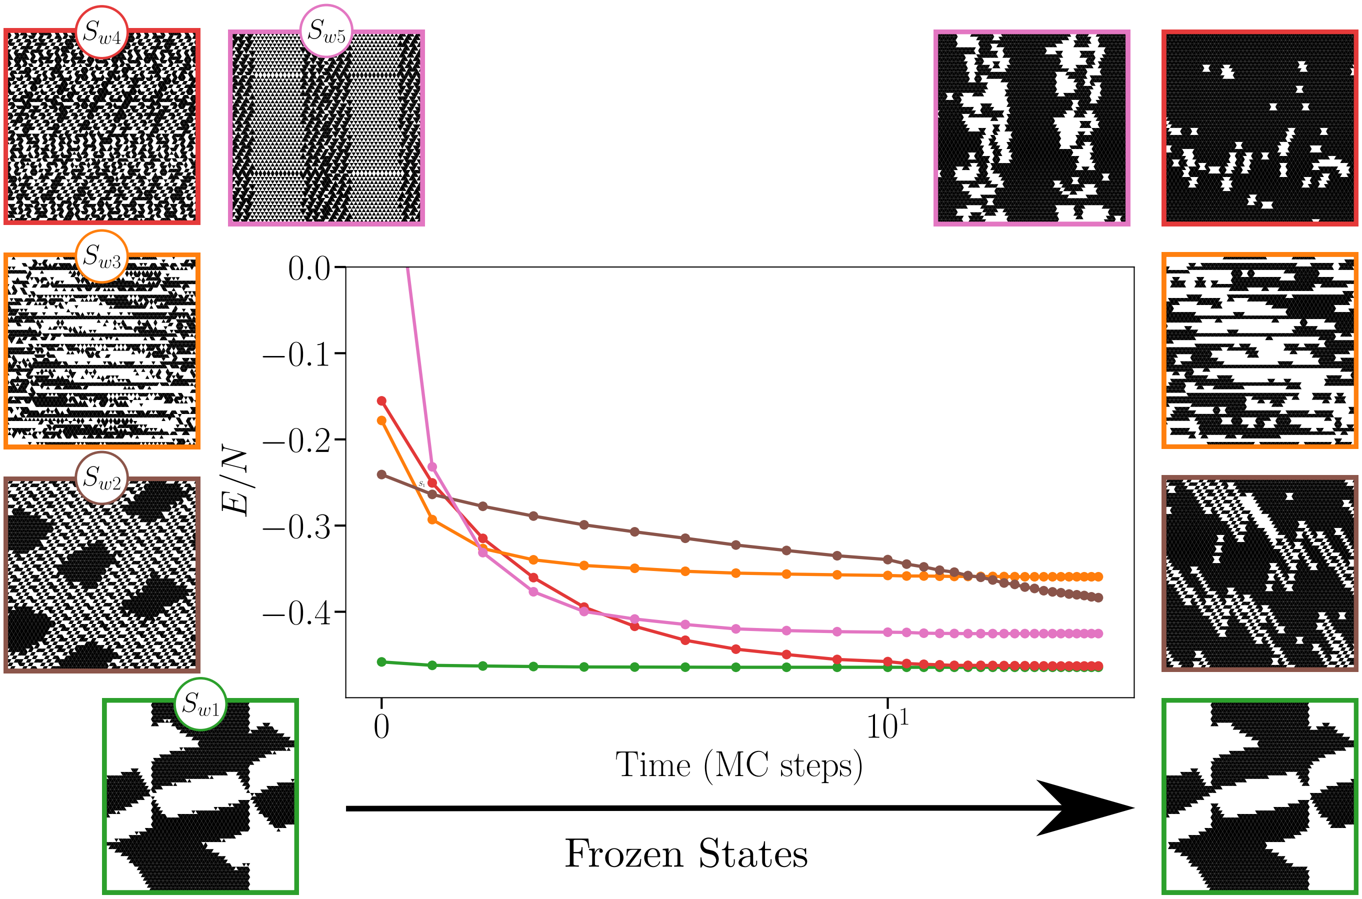


Figure 9. Temporal evolution and snapshots of the composition with weights of Chladni states for the hexagonal lattice of size $N = L_1 \times L_2 = 56 \times 86 = 5376$. The different states consist of the following combinations: $|S_{w1}\rangle = {}^1\!/_{10}\,|\lambda_2\rangle + {}^1\!/_5\,|\lambda_4\rangle + {}^3\!/_{10}\,|\lambda_8\rangle + {}^1\!/_{10}\,|\lambda_{16}\rangle + {}^3\!/_{10}\,|\lambda_{32}\rangle$, $|S_{w2}\rangle = {}^3\!/_{10}\,|\lambda_{17}\rangle + {}^1\!/_5\,|\lambda_{22}\rangle + {}^1\!/_2\,|\lambda_{1792}\rangle$, $|S_{w3}\rangle = {}^3\!/_{20}\,|\lambda_8\rangle + {}^{11}\!/_{50}\,|\lambda_{453}\rangle + {}^3\!/_{20}\,|\lambda_{345}\rangle + {}^7\!/_{25}\,|\lambda_{1234}\rangle + {}^1\!/_5\,|\lambda_{3485}\rangle$, $|S_{w4}\rangle = {}^1\!/_5\,|\lambda_{756}\rangle + {}^3\!/_{10}\,|\lambda_{1812}\rangle + {}^1\!/_2\,|\lambda_{2016}\rangle$ and $|S_{w5}\rangle = {}^3\!/_{25}\,|\lambda_{12}\rangle + {}^9\!/_{25}\,|\lambda_{3196}\rangle + {}^{12}\!/_{25}\,|\lambda_{5370}\rangle$.

### Supercrystal lattice

We have also analyzed a 2D lattice based on a specific underlying mesoscopic arrangement, known as Supercrystals (SCs), observed in a large variety of ferroelectric and other functional materials (we refer to [5] for further details). This lattice corresponds to a square-octagon lattice and is a special case of a two-scale lattice.

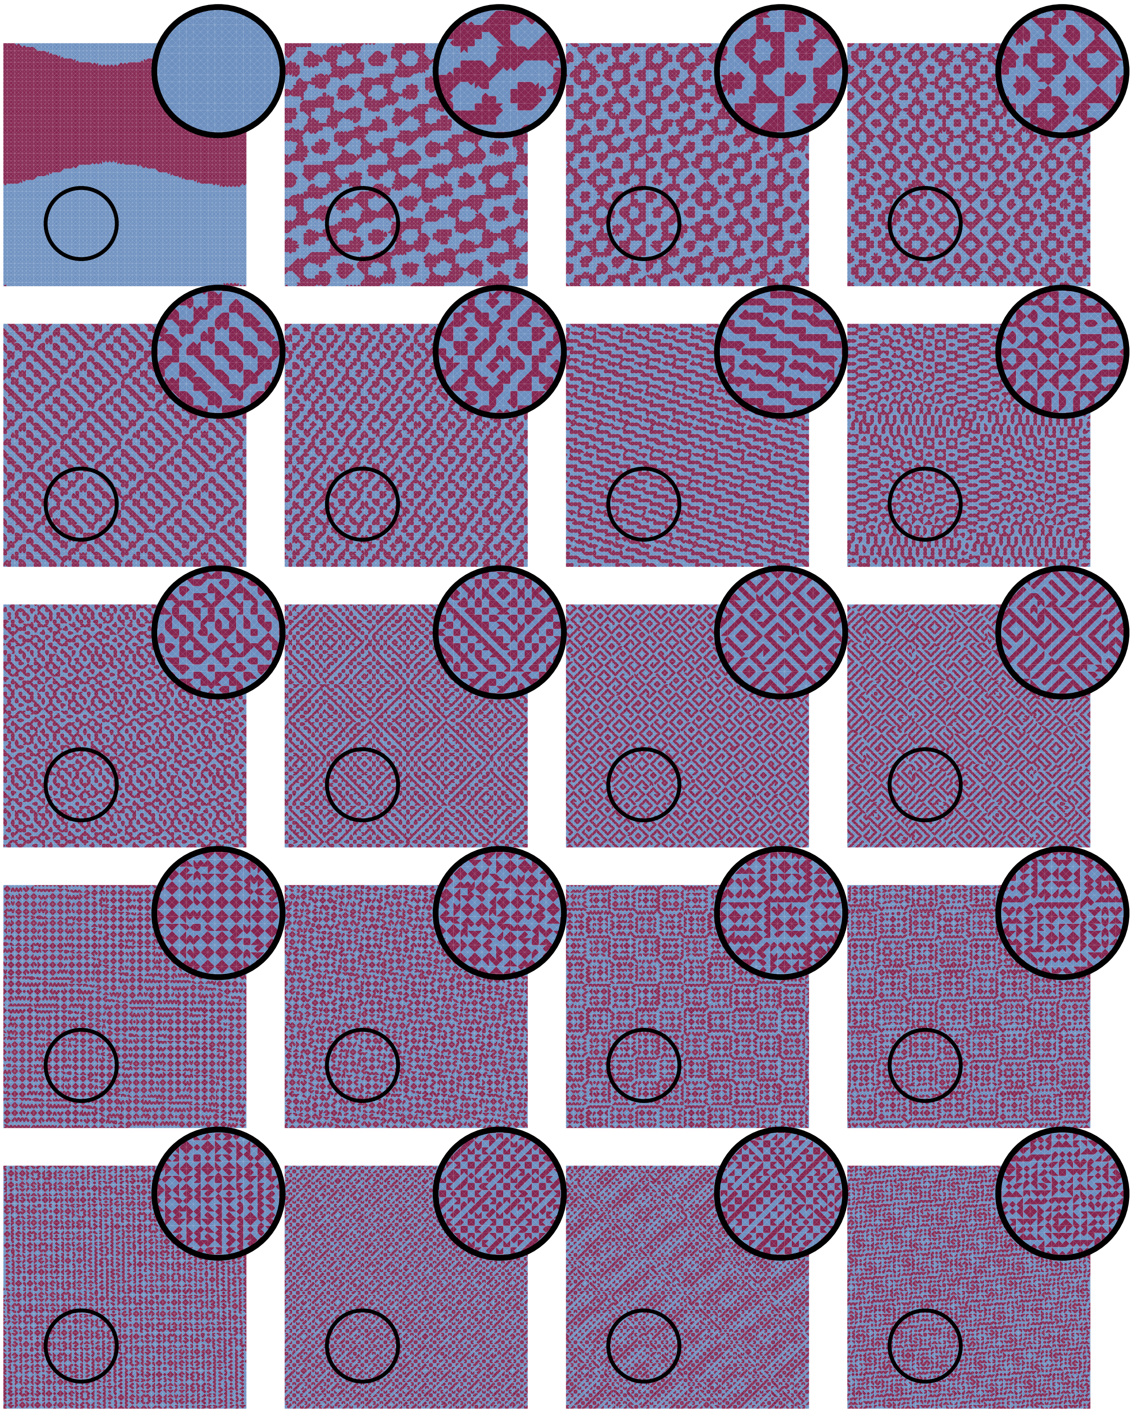

Figure 10. Chladni states for a 2D Supercrystal structure with side $L = 64$ (i.e. $N = 4 \cdot L^2 = 16384$) associated with different eigenvectors (in order, from top left corner to bottom right one: {1, 432, 863, 1294, 1725, 2156, 2587, 3018, 3449, 3880, 4312, 4743, 5174, 5605, 6036, 6467, 6898, 7329, 7760, 8192}. Zoomed regions illustrate the microscopic structure of complex patterns and different domain walls.

Figure 11 shows the energy corresponding to each normalized Chladni state as a function of the normalized growing eigenvectors. The energy curve exhibits symmetry about the origin, as it is able to sustain an antiferromagnetic phase. Note that the vibrational spectrum shows new symmetries and characteristic scales: a large-scale effective square lattice that starts to combine with the microscopic scale, giving rise to different Chladni states. We have performed extensive Monte Carlo simulations of selected Chaldni states at $T = 0$ to monitor their temporal evolution and analyze their stability, as reported in Fig. 11. In particular, we observe that such states associated with low lattice eigenmodes (or large spatial scales) exhibit negative energy and are temporally stable, i.e., the system remains stuck. However, those that correspond to the new introduced scale, i.e., over $i/N > 0.25$, are not stable in this specific case (see Fig. 11).

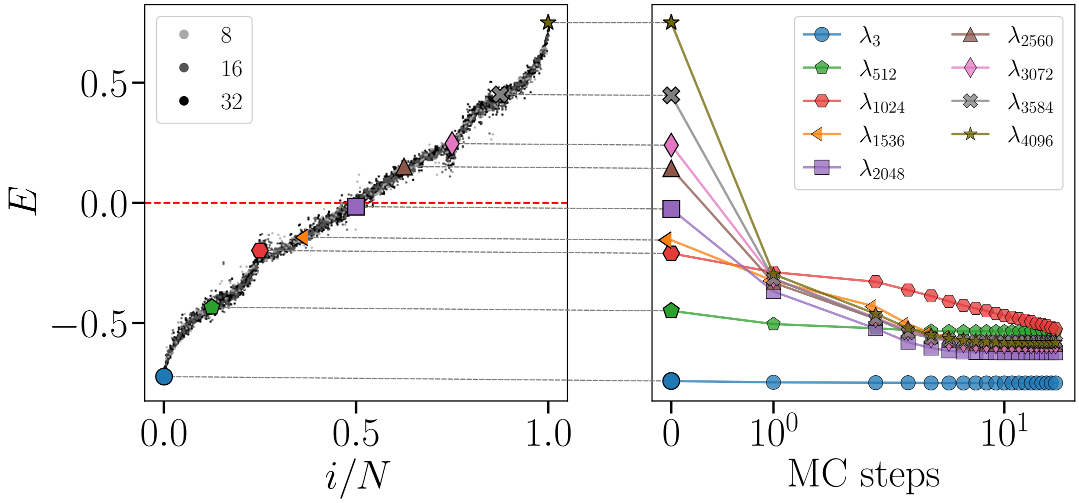


Figure 11. **Chladni states in 2D Supercrystal lattices.** **(Left)** Ising energy versus normalized eigenstate number for different system sizes (see legend, $N = 4 \cdot L^2$). Note the natural collapse of the curve for all lattice sizes. The red dashed line indicates zero energy. **(Right)** Temporal evolution at $T = 0$ of the different Chladni states versus time (in MC steps) for selected configurations (see legend) and energy mapping (dashed lines). Chladni states with enough negative energy define stable configurations over time.

**FRUSTRATED ANTIFERROMAGNETIC LATTICES AT ZERO TEMPERATURE.**

Figure 12 shows the energy corresponding to each normalized Chladni state as a function of the normalized growing eigenvectors for a 2D triangular antiferromagnetic lattice, being independent of the system size. Note that the energy curve does not exhibit symmetry about the origin (it is a mirroring of the curve shown before), as a consequence of the lack of an antiferromagnetic phase in this case. Again, Chladni states with negative energy are stable over time at $T = 0$.

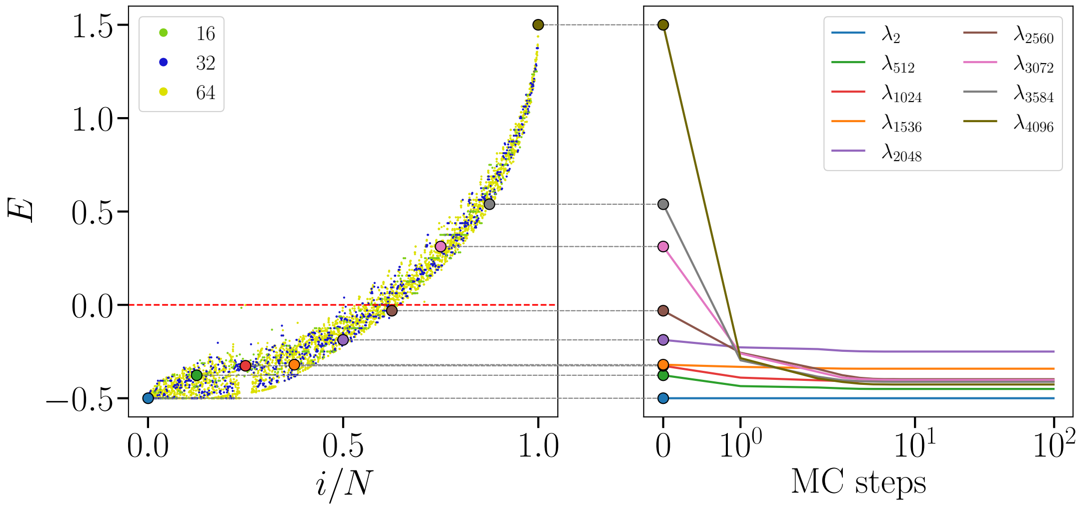


Figure 12. **Chladni states in 2D triangular antiferromagnetic lattices. (Left)** Ising energy versus normalized eigenstate number for different system sizes (see legend, $N = L^2$). The red dashed line indicates zero energy. **(Right)** Temporal evolution of the different Chladni states at $T = 0$ versus time (in MC steps) for selected configurations (see legend) and energy mapping (dashed lines). Chladni states with enough negative energy define stable configurations over time.

Figure 13 reports the combination of different Chladni states $\widetilde{|\lambda_i\rangle}$ for the 2D triangular lattice via weighted sum, $|w\rangle = \sum_i c_i |\lambda_i\rangle$, and element-wise product, and their temporal evolution considering the kinetically-constrained dynamics at zero temperature. During evolution, the system retains memory of structures stemming from negative-energy regions (see, for instance, the pink line in Fig. 13). Note that the decay to an equilibrium state depends on the original combination of Chladni states (see brown line in Fig. 13).

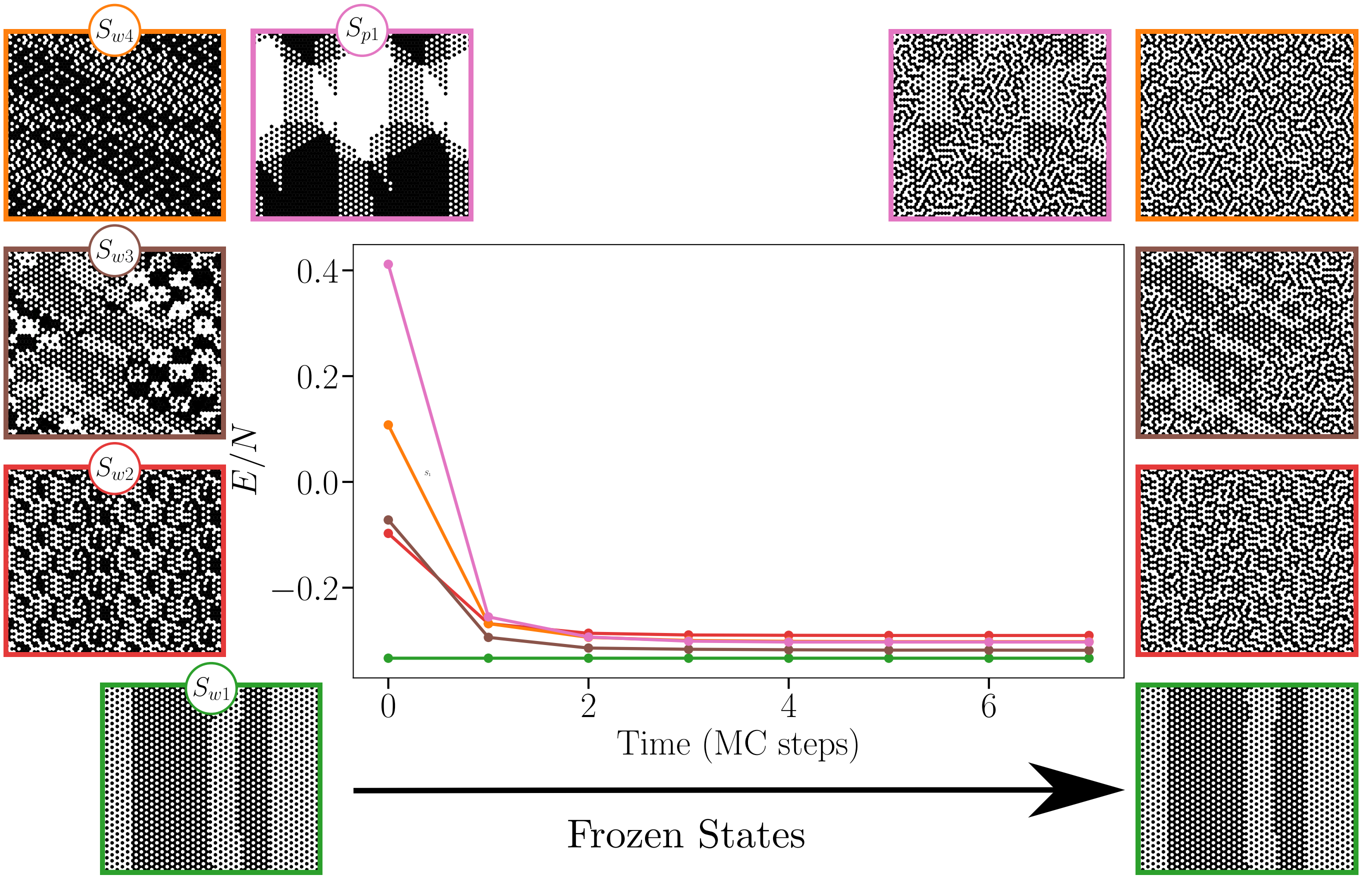


Figure 13. Temporal evolution and snapshots of the composition with weights of Chladni states for the antiferromagnetic triangular lattice of size $N = 64^2 = 4096$. The different states consist of the following combinations: $|S_{w1}\rangle = {}^{33}/_{100}\,|\lambda_0\rangle + {}^{33}/_{100}\,|\lambda_1\rangle + {}^{33}/_{100}\,|\lambda_2\rangle$, $|S_{w2}\rangle = {}^{1}/_{4}\,|\lambda_3\rangle + {}^{1}/_{2}\,|\lambda_{456}\rangle + {}^{1}/_{4}\,|\lambda_{789}\rangle$, $|S_{w3}\rangle = {}^{3}/_{10}\,|\lambda_4\rangle + {}^{23}/_{100}\,|\lambda_{18}\rangle + {}^{1}/_{5}\,|\lambda_{2560}\rangle + {}^{27}/_{100}\,|\lambda_{3894}\rangle$, $|S_{w4}\rangle = {}^{1}/_{2}\,|\lambda_4\rangle + {}^{1}/_{2}\,|\lambda_{1200}\rangle$ and $|S_{p1}\rangle = |\lambda_2\rangle \odot |\lambda_8\rangle$.

## SPIN-GLASS SYSTEMS

Figure 14 shows the energy corresponding to each normalized Chladni state as a function of the normalized growing eigenvectors for a 2D hexagonal lattice on the spin-glass phase ($p = 0.2$, with $p > p_c \simeq 0.064$), being independent of the system size. Note that the energy curve becomes linear and exhibits trivial symmetry about the origin. Again, Chladni states with negative energy are stable over time at $T = 0$.

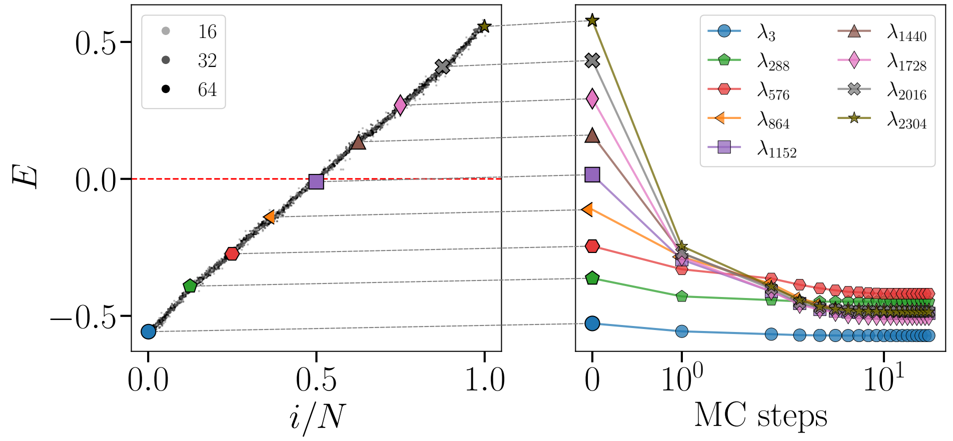


Figure 14. **Chladni states in a 2D glassy Hexagonal Lattice. (Left)** Ising energy versus normalized eigenstate number for different system sizes (see legend, $N = L_1 \cdot L_2$, where $L_1 = \sqrt{3}/2L_2$) and $p = 0.2$. Note the natural collapse of the curve for all lattice sizes. The red dashed line indicates zero energy. **(Right)** Temporal evolution at $T = 0$ of the different Chladni states versus time (in MC steps) for selected configurations (see legend) and energy mapping (dashed lines). Chladni states with enough negative energy define stable configurations over time.

Figure 15 shows the reconstructability index for different values of $p$ and $T$, which exhibits a clear shift at the paramagnetic phase, confirming its predictive power in identifying the loss of mesoscopic order in short-range spin-glass models.

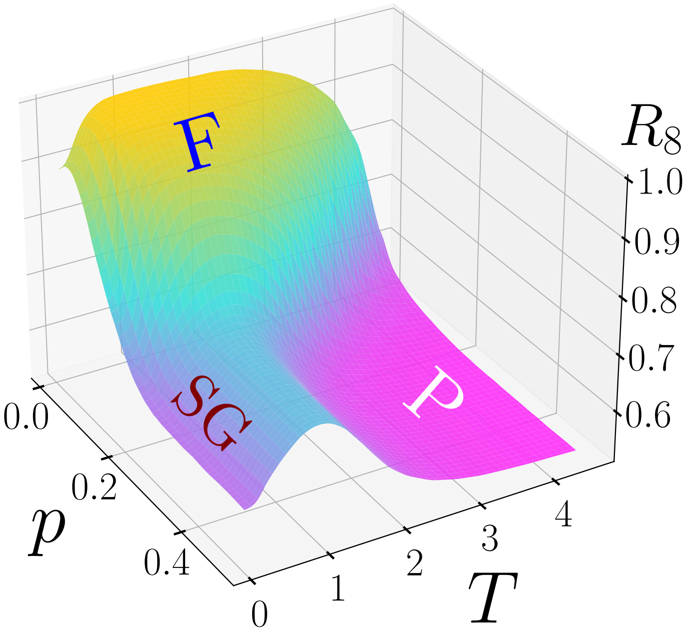


Figure 15. Three-dimensional reconstructability phase diagram using the top three eigenmodes, $R_3$, for a 3D cubic spin-glass lattice as a function of $p$ and $T$. The spin-glass phase emerges at $T = 0$ for $p_c = 0.22$, and the point $T = 1$ corresponds to the emergence of the paramagnetic phase for $p \gg p_c$.

**TOPOLOGICAL RECONSTRUCTION OF IMAGES**

We begin with a generic connected weighted graph $G = (V, E)$ on $N$ nodes, where each edge weight $w_{ij} \in \mathbb{R}$ may be positive or negative. The signed Laplacian, $\bar{L} = |D| - J$, accounts for both attractive and repulsive couplings, and has been shown to capture the topological features of frustrated interactions [1]. Now, $D = \sum_j |J_{ij}|$ represents the (absolute) weighted degree of each site. Once more, we describe here the most general case, as the signed Laplacian is formally equal to the Laplacian matrix, $L = D - A$, when all the entries have positive weights.

The cornerstone of our method is the eigendecomposition of $\bar{L}$, namely

$$\bar{L}_s\, \phi_k = \lambda_k\, \phi_k,$$

with $0 \leq \lambda_1 \leq \cdots \leq \lambda_n$ and orthonormal eigenvectors $\{\phi_k\}_{k=1}^{n}$. Putting these into $\Phi = [\phi_1, \ldots, \phi_n]$ yields $\Phi^\top \Phi = I$. An input signal $x \in \mathbb{R}^n$ is encoded by projection onto this spectral basis:

$$z = \Phi^\top\, x \in \mathbb{R}^n,$$

so that $z_k$ measures the content of $x$ in the $k$-th (un)signed-graph frequency.

To extract class-specific information, we define, for each class $c$, the average spectral encoding over its training examples,

$$\mu_c = \frac{1}{|\mathcal{D}_c|} \sum_{x_i \in \mathcal{D}_c} \Phi^\top\, x_i,$$

where $\mathcal{D}_c$ denoting the training subset corresponding to class $c$. Each $\mu$ is then centered and normalized:

$$\widetilde{\mu}_c = \frac{\mu_c - \overline{\mu}_c}{\|\mu_c - \overline{\mu}_c\|_2},$$

where $\bar{\mu}_c$ is the empirical mean over classes. For an $M$-way classification task, we have the transformation matrix,

$$P = \begin{pmatrix} \widetilde{\mu}_{c_1}^\top \\ \widetilde{\mu}_{c_2}^\top \\ \vdots \\ \widetilde{\mu}_{c_3}^\top \end{pmatrix} \in \mathbb{R}^{M \times n}.$$

For example, for the three-digit classification task introduced in the main document (digits $1, 2, 3$), $P$ explicitly takes the form

$$P = \begin{pmatrix} \widetilde{\mu}_{1,1} & \widetilde{\mu}_{1,2} & \cdots & \widetilde{\mu}_{1,n} \\ \widetilde{\mu}_{2,1} & \widetilde{\mu}_{2,2} & \cdots & \widetilde{\mu}_{2,n} \\ \widetilde{\mu}_{3,1} & \widetilde{\mu}_{3,2} & \cdots & \widetilde{\mu}_{3,n} \end{pmatrix},$$

where each row corresponds to the centered unit norm instance of one-digit class.

Any new input $x$ is thus mapped to an $M$-dimensional embedding, namely,

$$h = P\, z \;=\; P\, (\Phi^\top x) \;\in \mathbb{R}^M,$$

whose components $h_c$ quantify similarity to class $c$. Although a full decoder architecture is not the focus here, one may easily perform a reconstruction map $W \in \mathbb{R}^{n \times M}$ by minimizing

$$\|x - W\, h\|_2^2 \;+\; \alpha\, h^\top \bar{L}\, h.$$

**The reconstruction of an image.** Figure 17 shows the reconstruction of a selected image (as shown in Fig. 16) using a square lattice, an antiferromagnetic triangular lattice, and a 3D cubic lattice.

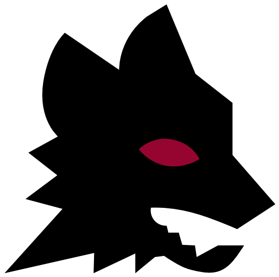

Figure 16. Original image.

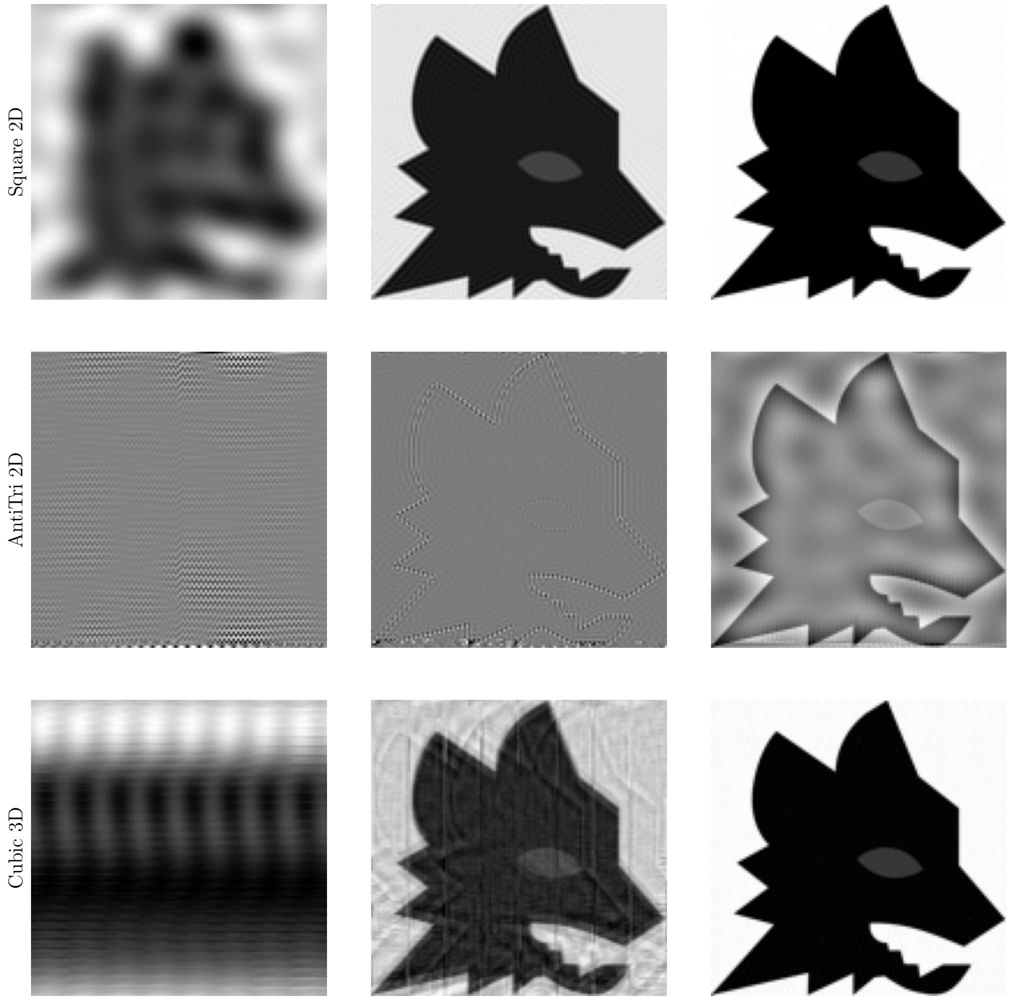


Figure 17. Reconstructed image using the first 100 (left column), $N/2$ (central column), and $N-100$ (right column) eigenvectors for a 2D square lattice, a 3D cubic lattice ($N = 32 \cdot 32 \cdot 16$, projected onto a 2D structure), and an antiferromagnetic triangular lattice.

Figure 18 shows the reconstruction of a particular MNIST digit using different architectures. In particular, we have used 2D lattices, including the squared, triangular, and hexagonal lattices, as well as a 3D cubic lattice, a 3D cubic lattice in the spin-glass phase, and an Erdős–Rényi networks. As shown in the main text, in the case of a $2d$ image, clearly, the best embedding would be achieved with a simple bidimensional square lattice. One can easily notice how, depending on the structure, this number is highly variable, focusing attention on selecting the appropriate topology for the specific dataset.

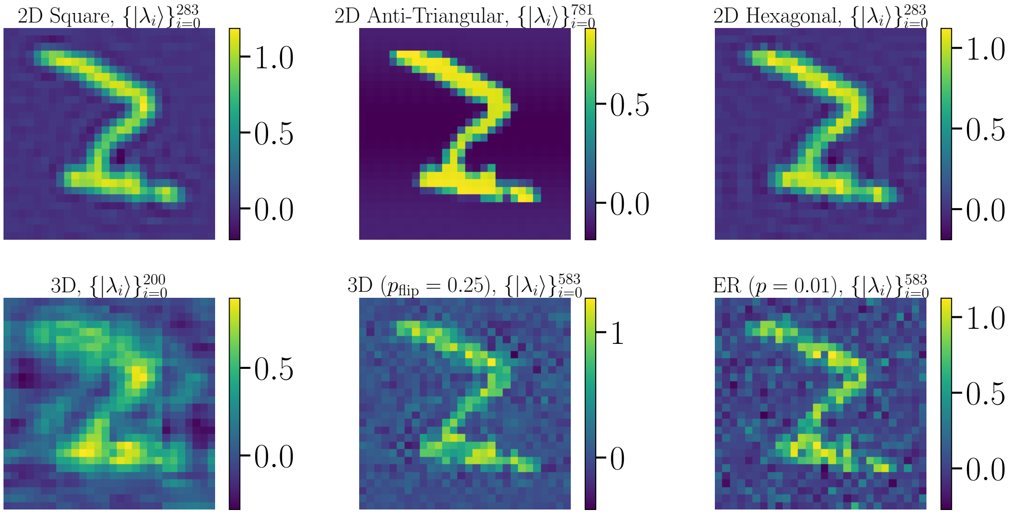


Figure 18. Reconstruction of a MNIST digit using the first $k$ eigenvectors for different topological structures, where $k$ is specified by the corresponding number in each sub-figure title. One can easily notice how, depending on the structure, this number is highly variable, focusing attention on selecting the appropriate topology for the specific dataset. In the case of a $2d$ image, clearly, the best embedding would be achieved with a simple bidimensional square lattice.

[1] G. Iannelli, P. Villegas, T. Gili, and A. Gabrielli, arXiv preprint arXiv:2504.00144 (2025).
[2] D. J. Amit and V. Martin-Mayor, *Field Theory, the Renormalization Group, and Critical Phenomena*, 3rd ed. (World Scientific, Singapore, 2005).
[3] J. J. Binney, N. J. Dowrick, A. J. Fisher, and M. E. Newman, *The theory of critical phenomena: an introduction to the renormalization group* (Oxford University Press, Oxford, 1992).
[4] Y. Liu and J. Shen, Taiwanese J. Math. **19**, 505 (2015).
[5] L. Falsi, P. Villegas, T. Gili, A. J. Agranat, and E. DelRe, arXiv , 2406.14646 (2024).
